# Supplementary material for: Stein Variational Gradient Descent With Matrix-Valued Kernels
Source: arXiv:1910.12794 source file (2019-11-05)
Supplement: Supplementary file 1 [file appendix_qiang.tex]

%\appendix
